# Supplementary material for: Can I Trust My Simulation Model? Measuring the Quality of Business Process Simulation Models
Source: arXiv:2303.17463 source file (2023-03-30)
Supplement: Supplementary file 1 [file sm.tex]

ServiceMiner (SM) operates in three steps, namely data preprocessing, 
data enhancement, and model learning.
First, event data goes through preprocessing such as data cleaning, and 
dummy encoding of categorical features. For data enhancement, new data attributes that capture trend, and seasonality, as well as system congestion are created using methods described in~\cite{senderovich2019congestion}.
In the model learning step, SM uses three techniques: process discovery (the main
task of process mining), queue mining (learning of queueing building blocks from data), and 
machine learning (to boost the accuracy of arrival and activity time genration). For process discovery, SM mines a Markov chain, estimating the routing probabilities 
between pairs of nodes. An abstraction mechanism allows for filtering out of rare activities, paths, and transitions,
based on the created graph. Next, using queue mining, the various queueing building blocks are fitted from data. The basic version of queue mining is described in~\cite{senderovich2016conformance}; ServiceMiner uses advanced versions of these techniques.
The model that results from queue mining is a queueing network with Markovian routing. 
Lastly, we apply machine learning methodology that uses congestion related features that come from queueing theory,
which, via cross-validation, leads to accuracy improvements when generating arrival and activity duration.
